# Supplementary material for: Quantifying the Academic Quality of Children's Videos using Machine Comprehension
Source: arXiv:2303.17201 source file (2024-02-06)
Supplement: Supplementary file 1 [file appendix.tex]

\newpage
\appendices

\section{Additional Details on TQA Dataset}

To the best of our knowledge, TQA Dataset is the only dataset developed based on children's textbooks. The dataset has been sourced from ck12.org, which provides educational content to children. TQA Dataset, which consists of multiple topics like earth sciences, oceans, human biology, physics fundamentals, etc., Fig. 10 demonstrates the tree structure of the dataset within each topic; there are multiple sub-topics each of them will have context and related questions, and answers related to the sub-topic.

\begin{figure}[hb!]
    %\centering
    \includegraphics[width=0.48\textwidth]{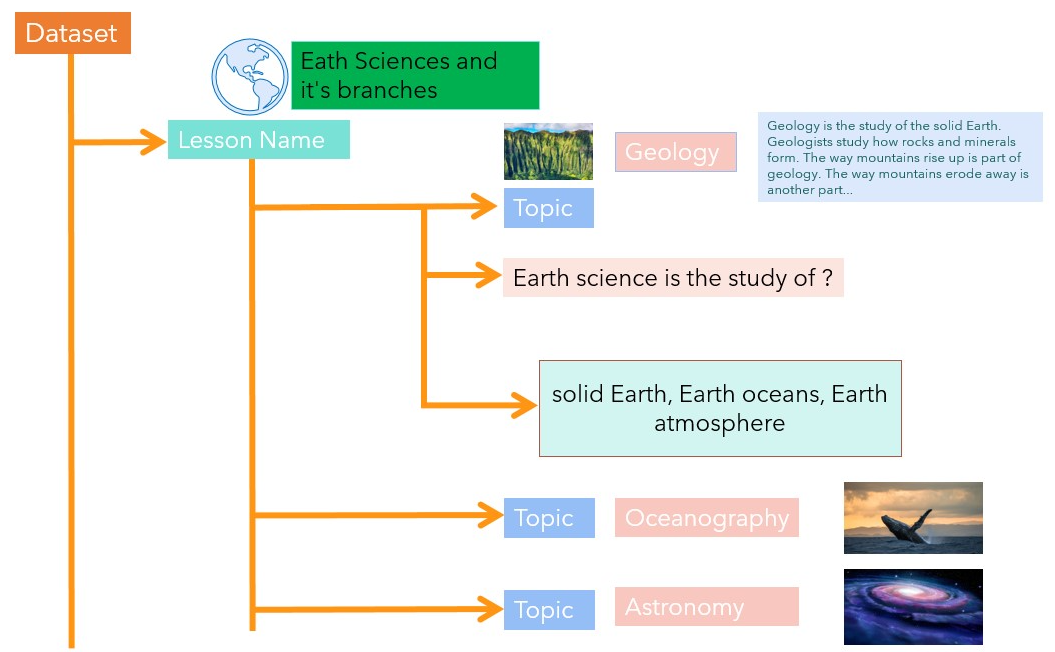}
    \caption[RC Model]{Tree structure of TQA Dataset, root node starts on the left.}
    \label{fig:tqa_details}
\end{figure}

Figure \ref{fig:tqa_details} shows how the QA dataset is arranged. TQA dataset comprises multiple lessons (e.g., Earth Sciences and its branches). Each lesson has multiple topics (like Geology, Oceanography) that contain some background context of the topic and related questions and answers.

 In Tbl.~\ref{tab:tqa_dataset}, we present a subset of this dataset, showing sample topics, 
the number of questions, topics, a sample question,  and a sample answer.
\begin{table}[ht!]
\scriptsize
\caption{TQA  Dataset}
\centering
\begin{tabular}{|p{1.7cm}|p{1.0cm}|p{0.8cm}|p{2.0cm}|p{1.0cm}|p{0.7cm}|p{0.7cm}|}
 \hline
 Sample Topic &  \# of Questions &  \# of Sub-Topics & Sample Question &   Sample Answer\\ [0.5ex] 
 \hline
 \hline
Earth science and its branches & 24 & 5 & A geologist would be most likely to investigate how & mountains form.\\\hline
Erosion and deposition by flowing water & 24 & 14 & More slowly flowing water can carry larger sediments. & false\\\hline
Erosion and deposition by waves & 24 & 10 & artificial barrier parallel to a shore that reduces beach erosion & breakwater\\\hline
Erosion and deposition by glaciers & 24 & 4 & Continental glaciers are long and narrow. & false\\\hline
Fossils & 40 & 10 & Fossilized insects have been found preserved in amber, which is hardened & tree sap \\\hline
 \end{tabular}
 \label{tab:tqa_dataset}
\end{table}

% % you can choose not to have a title for an appendix
% % if you want by leaving the argument blank
% \section{}
% Appendix two text goes here.
\section{Additional Details on Multi-modal Video Retriever}
The encoders are trained to make the similarity function a good ranking function during training. This is done  by encoding the topic and video representations of correct pairs closer to the encoding space than the irrelevant ones. To train the model, we use a contrastive learning approach. For training, we need the ground truth of positive and negative videos. Our dataset doesn't have such data, so we create pseudo-positive and negative videos using a BM25 retriever model based on the same video data. The videos that lead to correct answers are grouped as positives, while those that lead to incorrect answers are grouped as negatives for contrastive learning. Like the dense passage retriever paper, the loss function is the negative log-likelihood of the positive video data. Let $D_i = {⟨q_i, v_i^+ , v_{i,1}^-, · · · , v_{i,n}^-⟩}$ be the training data that consists of $m$ instances. Each instance contains one question $q_i$ and one relevant (positive) video $v_i^+$, along with n irrelevant (negative) videos $v_{i,j}^-$. For irrelevant negative videos, we consider top passages returned by the BM25 algorithm that does not contain the answer.

% \vspace{5}
\begin{equation}
    \begin{split}
    L(q_i, v^+_{(i,1)},v^+_{(i,2)},.. v^+_{(i,m)}, v^-_{(i,1)},v^-_{(i,2)},.. v^-_{(i,n)}) \\
    = - \sum^m_{k=1} log\frac{e^{sim(q_i,v^+_{(i,1)})}}{e^{ sim(q_i, v^+_{(i,1)})} + \sum^n_{j=1} e^{ sim(q_i, v^-_{(i,j)})}} 
    \end{split}
\end{equation}
% \vspace{5}

We use the gradient accumulation technique with eight accumulation steps and the AdamW optimization ~\cite{loshchilov2017decoupled} for model training. We use the PyTorch library to implement all the methods in this work. All experiments are conducted on one NVIDIA GTX 3090 GPU. 

% The hyperparameters considered in this paper are shown in Table 7.

\section{Additional Details on Pre-trained RC Models}

\begin{table}[htb!]
\scriptsize
\caption{Number of Parameters each model has}
\centering
\begin{tabular}{|p{2.7cm}|p{1cm}|}
 \hline
 Model &  \#Parameters \\ [0.5ex]
 \hline
 \hline
Longformer &  148M\\\hline
BiDAF &  12M \\\hline
BiDAF-ELMo & 113M\\\hline
Transformer QA & 355M\\\hline
 \end{tabular}
 \label{tbl:model_params}
\end{table}

We provide additional details on the pre-trained models. For Longformer, we have used the HuggingFace library\footnote{https://huggingface.co/transformers/v3.2.0/model\_doc/longformer.html}. For BiDAF, BiDAF-ELMo, and TransformerQA, we use Allennlp \footnote{https://docs.allennlp.org/models/main/} based pre-trained models. In Tbl. \ref{tbl:model_params} we have summarized the parameter size of each model. As we can observe, Transformer QA has the largest number of parameters, followed by the Longformer model. Despite the fewer parameters, the Longformer works better on our dataset (as shown in Experiment 1).

\begin{figure}[htb!]
    \centering
    \includegraphics[width=0.5\textwidth]{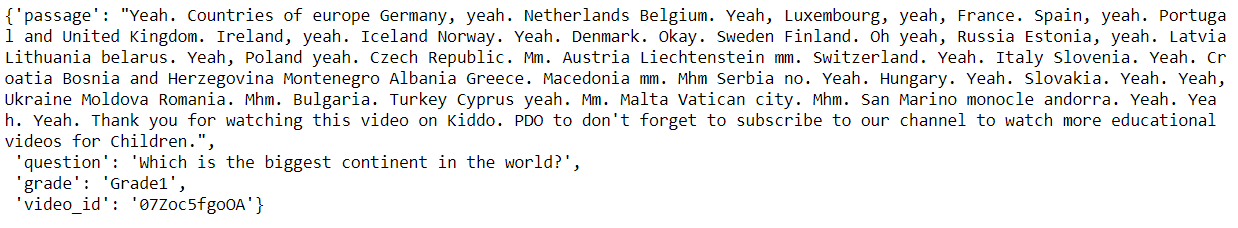}
    \caption[RC Model]{Sample input to the Bidaf-Elmo Model}
    \label{fig:input}
\end{figure}

The Allennlp-based models take input in a JSON format. Figure \ref{fig:input} demonstrates a sample input. The predict() method of the model only takes one sample passage and one question at a time and returns the answer in a string format. Therefore, we created JSON files combining the questions from the TQA Dataset and the text from the YouTube transcriptions and grouped them by channels.

% \begin{figure}[ht]
%     \centering
%     \includegraphics[width=0.5\textwidth]{IEEEtran/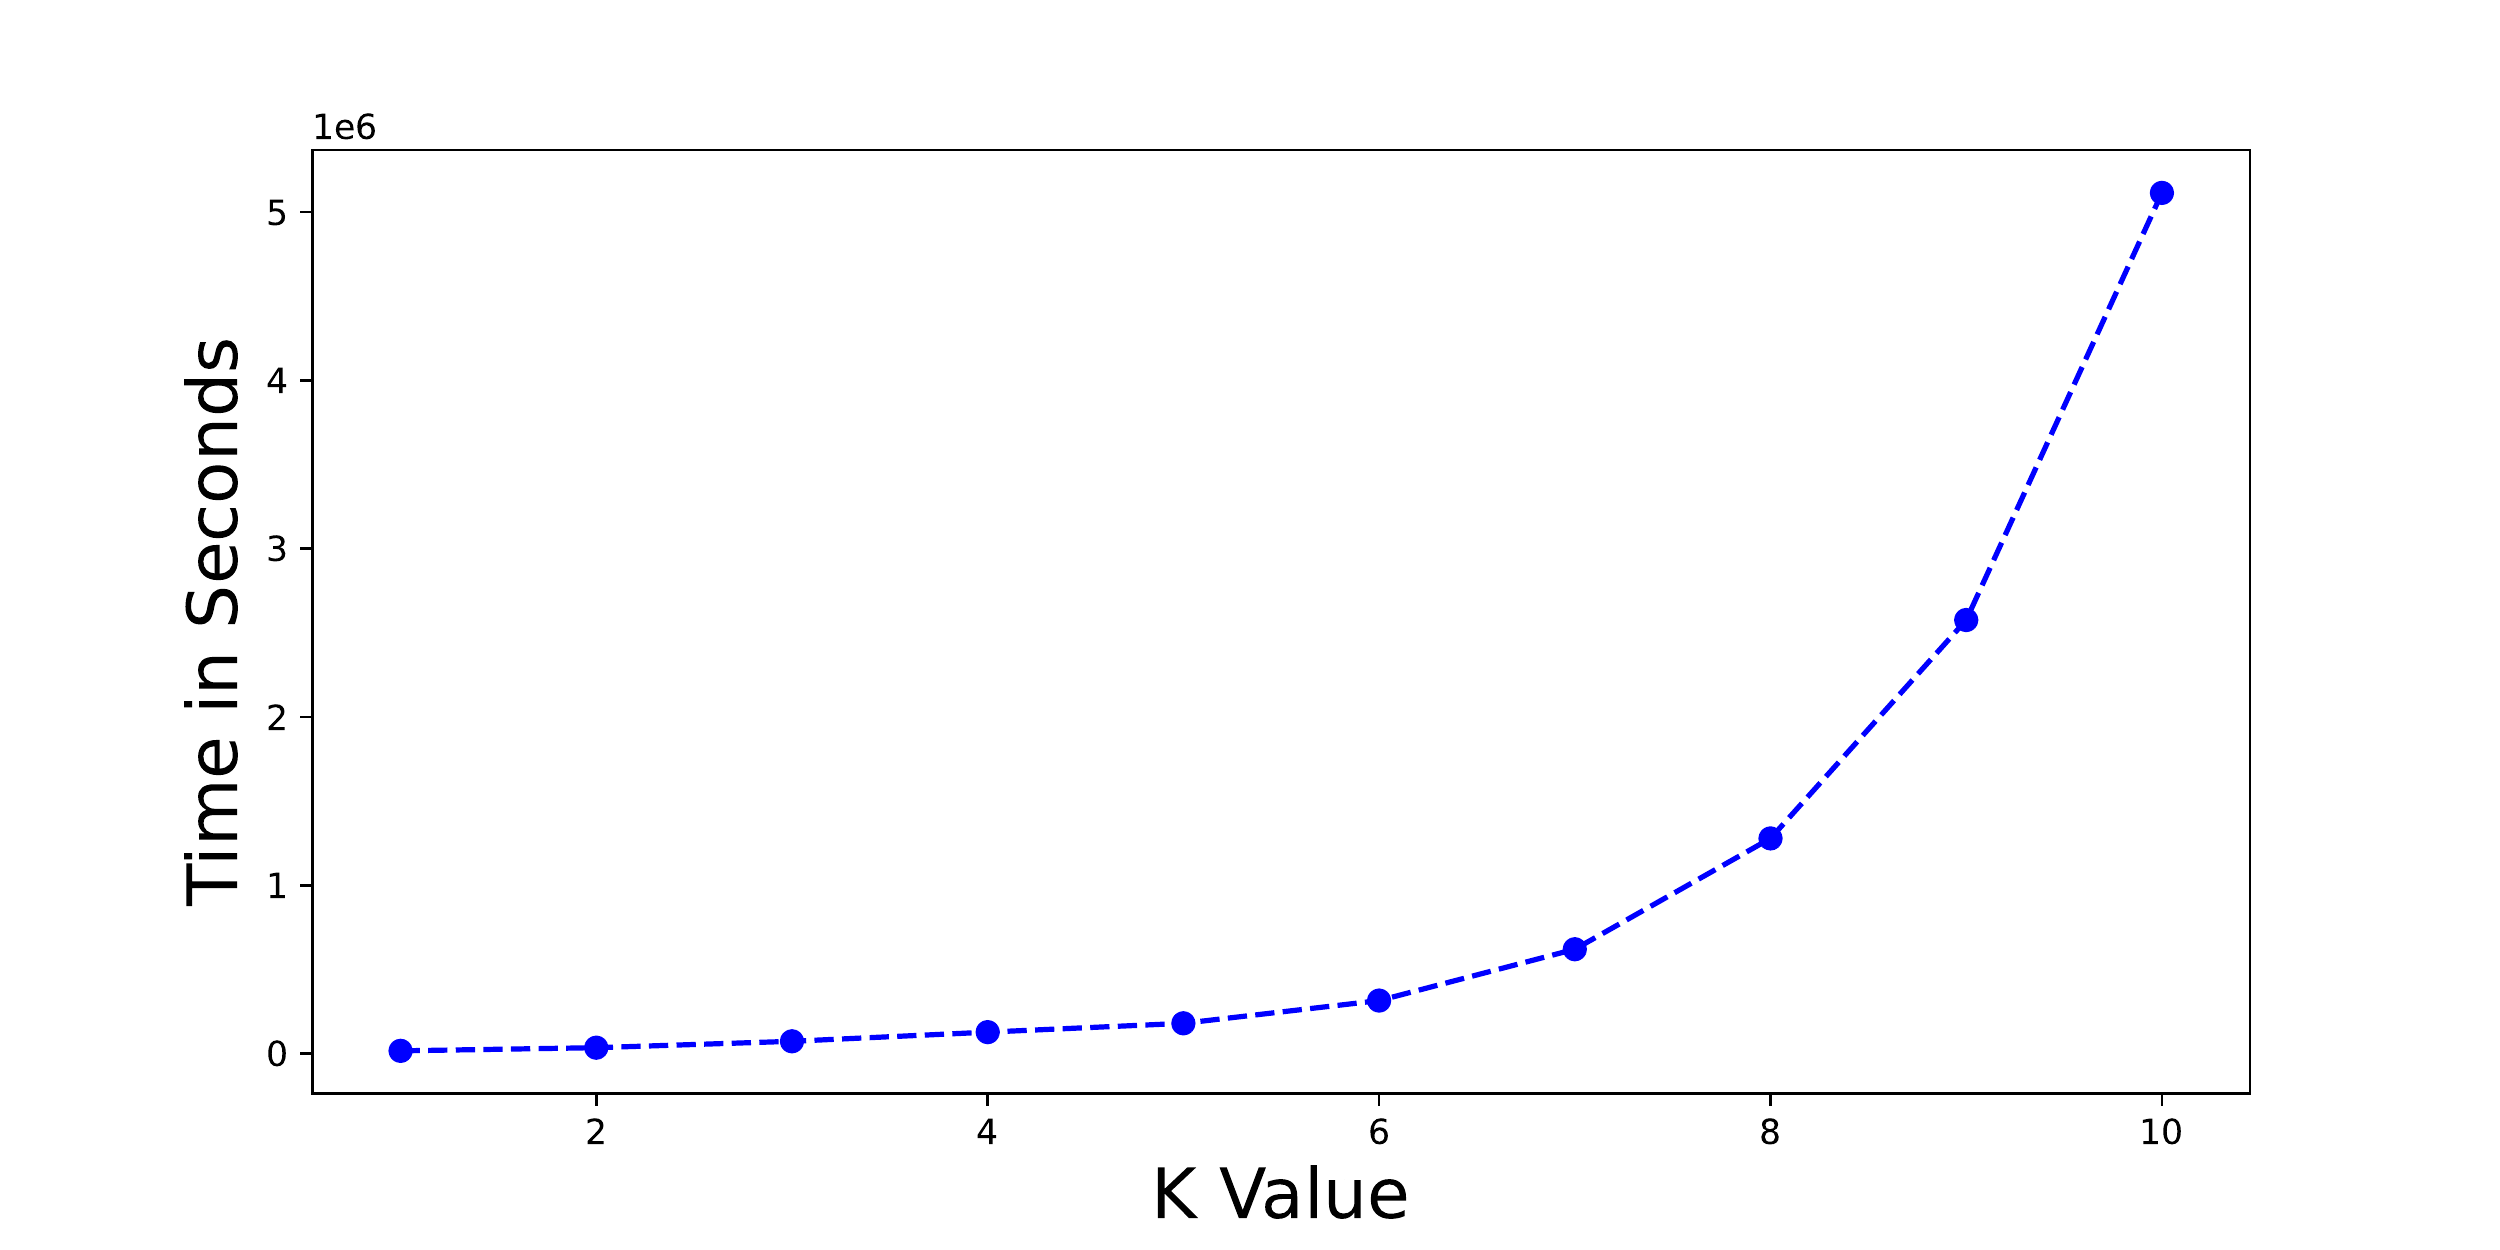}
%     \caption[RC Model]{Time complexity by changing with K values}
%     \label{fig:overall}
% \end{figure}
% In order to compare the predicted answer and the actual answer, we tokenized both the columns as they were of string type. Later on, we calculated the Jaccard Similarity between the predicted answer and the actual answer for each video ID grouped by channel ID. 

% $\mathcal{J}(\mathcal{A},\mathcal{B}) = \frac{|\mathcal{A} \cap \mathcal{B}|}{|\mathcal{A} \cup \mathcal{B}|}$

\section{Details on Video Labeling Exercise}
As there are no existing data sets on children's videos labeled for questions and answers, we created a small dataset of 100 videos, manually labeled for questions that can be answered using the information in the videos. We used the following filtration criteria for videos to label:
\begin{enumerate}
    \item Video should be publicly available and downloadable on YouTube  
    \item Video should have a video transcript that can be obtained using YouTube API
    \item Video should not be a live-streaming video
    \item Video sample should be from a diverse set of channels and video duration
\end{enumerate}

\begin{table}[htb!]
\scriptsize
\caption{Number of Questions in each Category}
\centering
\begin{tabular}{|p{1.5cm}|p{2cm}|}
 \hline
 Question Type &  No.of Questions \\ [0.5ex]
 \hline
 \hline
Simple &  502\\\hline
Complex &  120 \\\hline
 \end{tabular}
 \label{tbl:model_params}
\end{table}

Using the above condition, we selected a sample of 100 videos. The labeling was conducted by research assistants well-versed in English and a faculty member associated with a large private university. The labelers were provided a guideline document to label videos, asking them to review them individually. They should see the video and use the information (visuals and language) to form factual questions. In particular, think of questions that can be present in the school curriculum and could be asked in an academic exam. We also ask them to rate the video in terms of overall academic quality on a scale of five. These scores could be used in future work to correlate the video quality based on the labeler's score and the score obtained by the proposed ML model. Next, we provide more details on the labeling parameters. Each labeler was elaborated on the labeling exercise and was asked to provide the following information:
\begin{enumerate}
    \item Video\_id: The video id of the labeled YouTube video. The video-id is a unique identifier that identifies video on the YouTube platform and is not likely to change.
    \item Time: The approximate time in seconds when the question and answer were presented in the video. This information is not currently used in the analysis but could be later used in future work.
    \item Question: What's the factual question that can be answered?
    \item Question type (simple, complex): Is the question simple or complex? A simple question is one with the answer in the same sentence. A complex question is one that requires multiple sentences to be analyzed to retrieve the answer.
    \item Answer Modality (visual/language/both): The modality in which the answer is present. We provide samples of question-answers for the different types of modalities in Figs. \ref{fig:language_uestion}, \ref{fig:visual_example}, \ref{fig:dual_example}.
    \item Overall\_academic\_quality (1=very poor, 2, poor, 3=average, 4=high, 5=very high): Finally, the labeler was asked to provide the overall academic quality of the video (not per question).
\end{enumerate}

\begin{figure}[t]
    \centering
    \includegraphics[width=0.42\textwidth]{./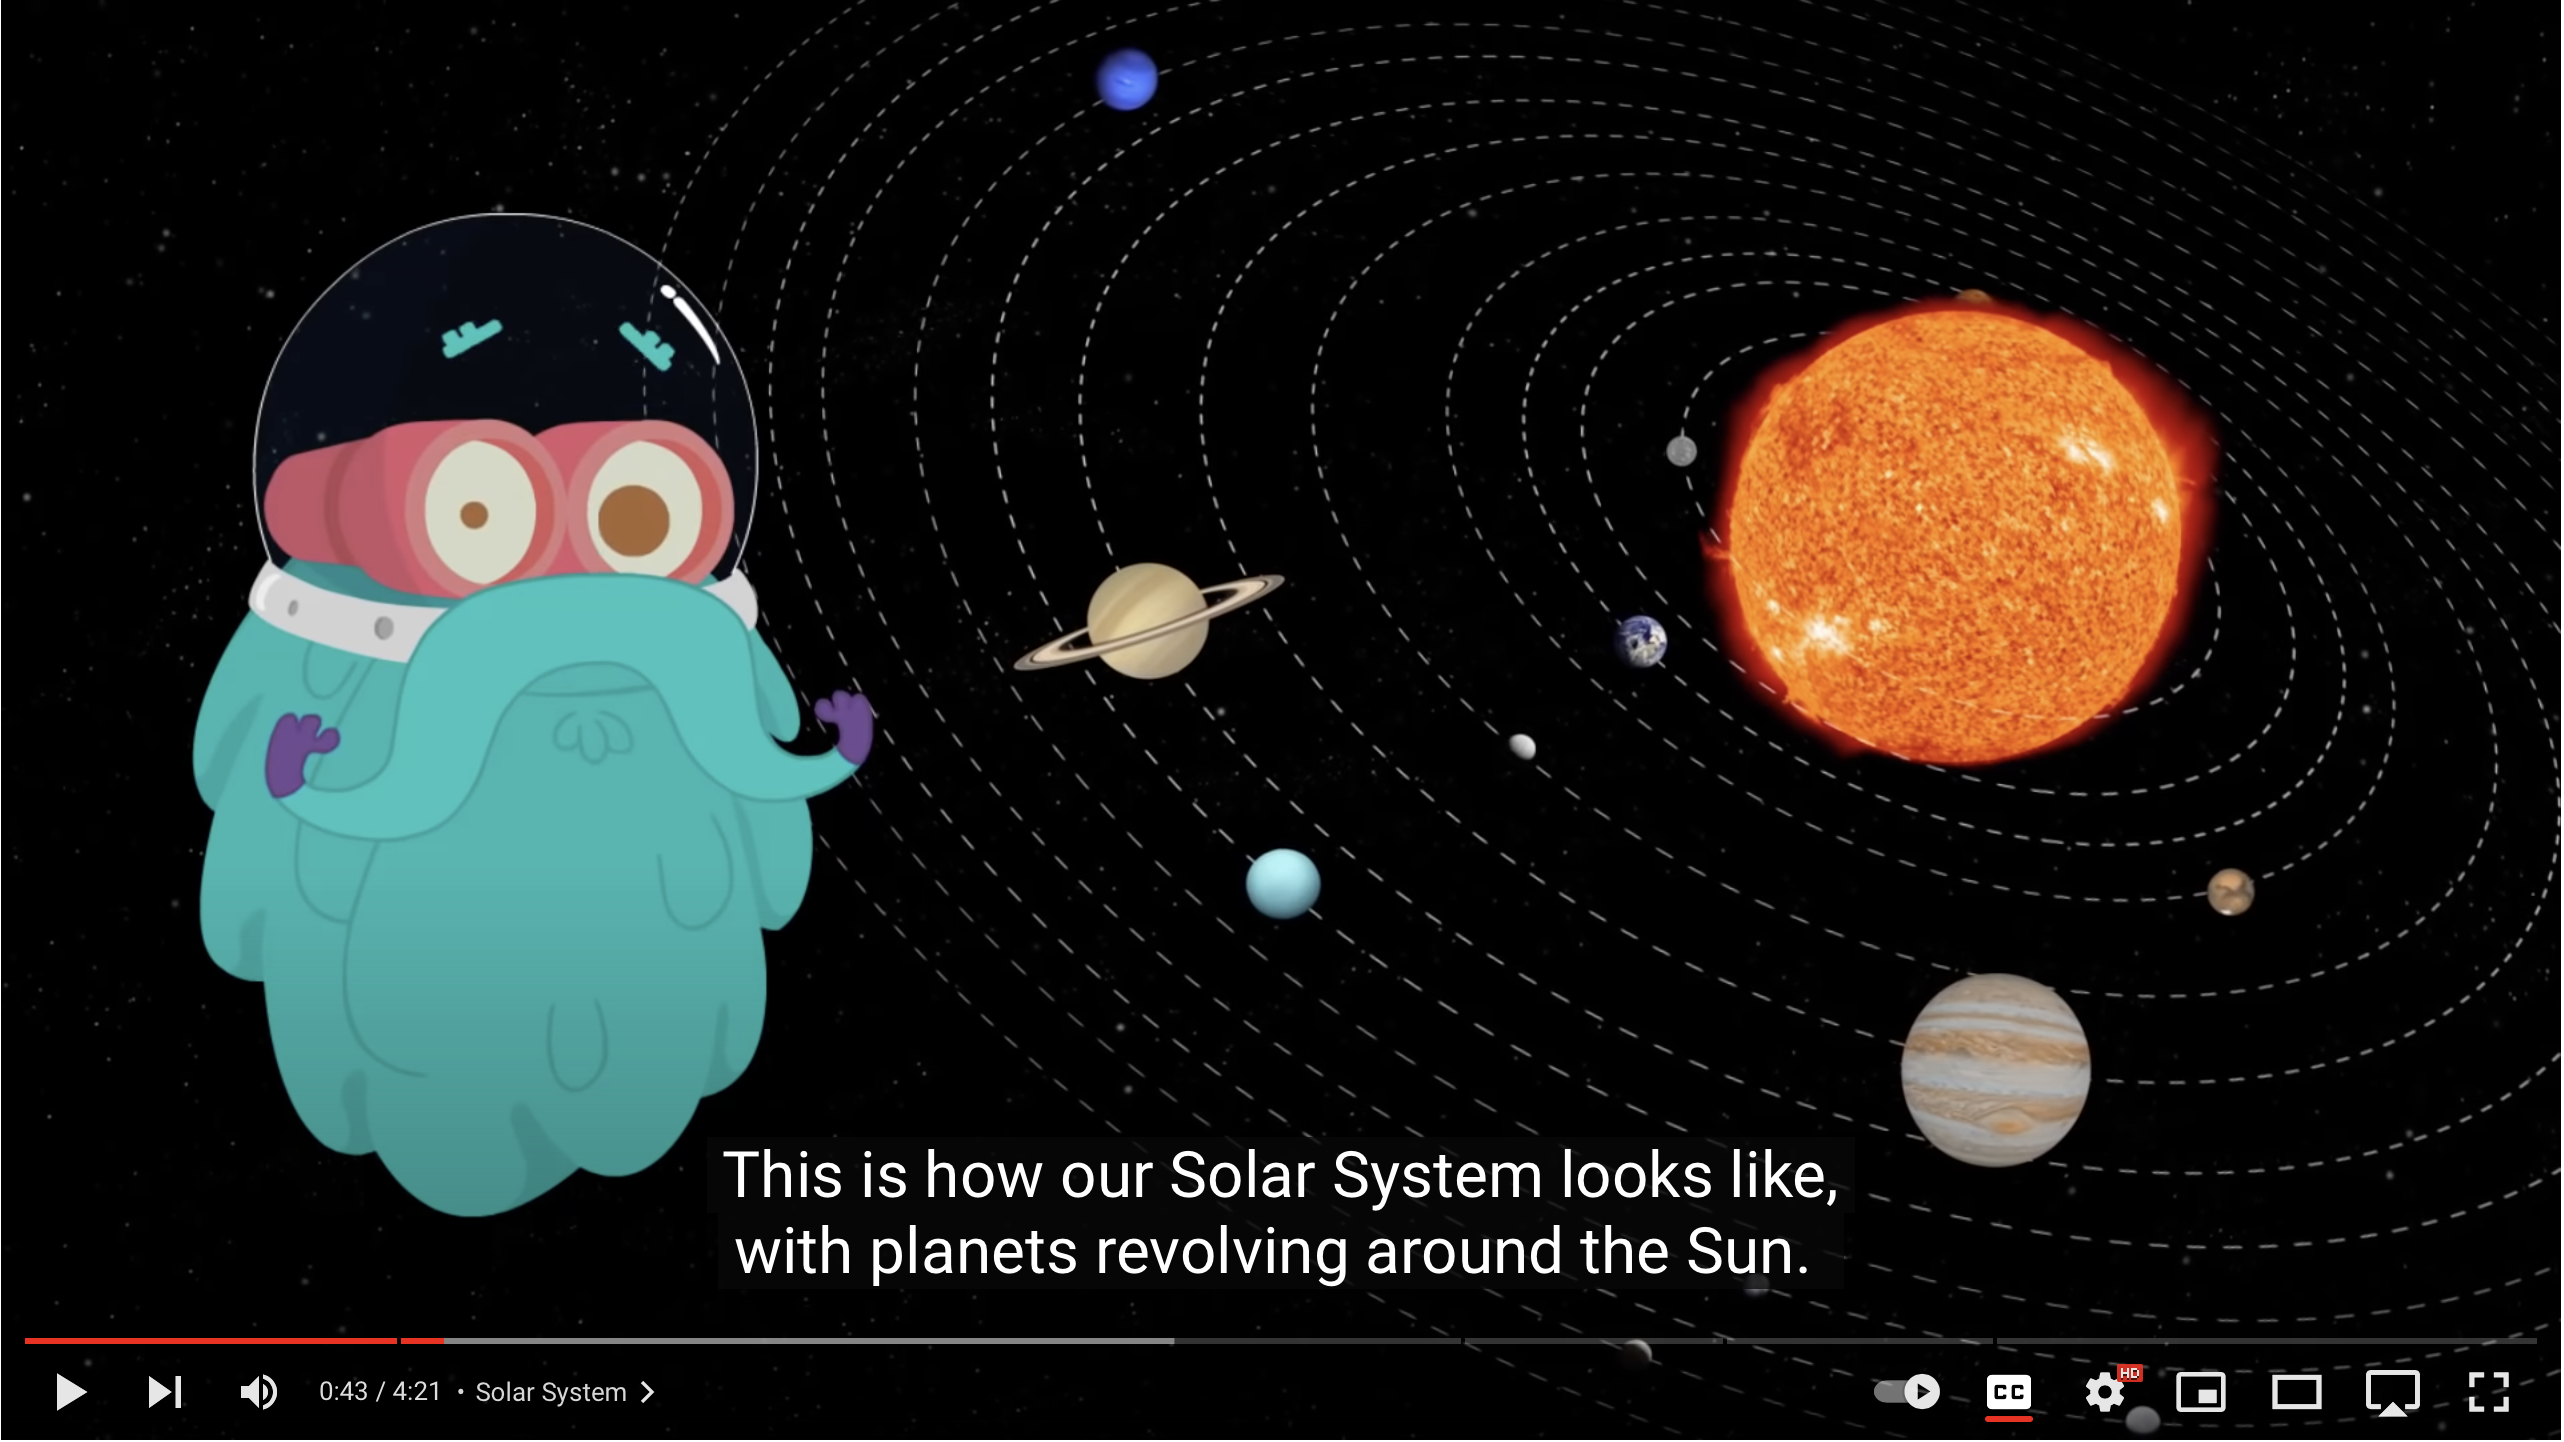}
    \caption[RC Model]{An example of a video-frame from a \textit{YouTube Kids} video explaining the Solar System. The video has information present in language modality (video transcription) to answer the question: `What revolves around the Sun?'}
    \label{fig:language_uestion}
\end{figure}

\begin{figure}[htb!]
    %\centering
    \includegraphics[scale=0.24]{./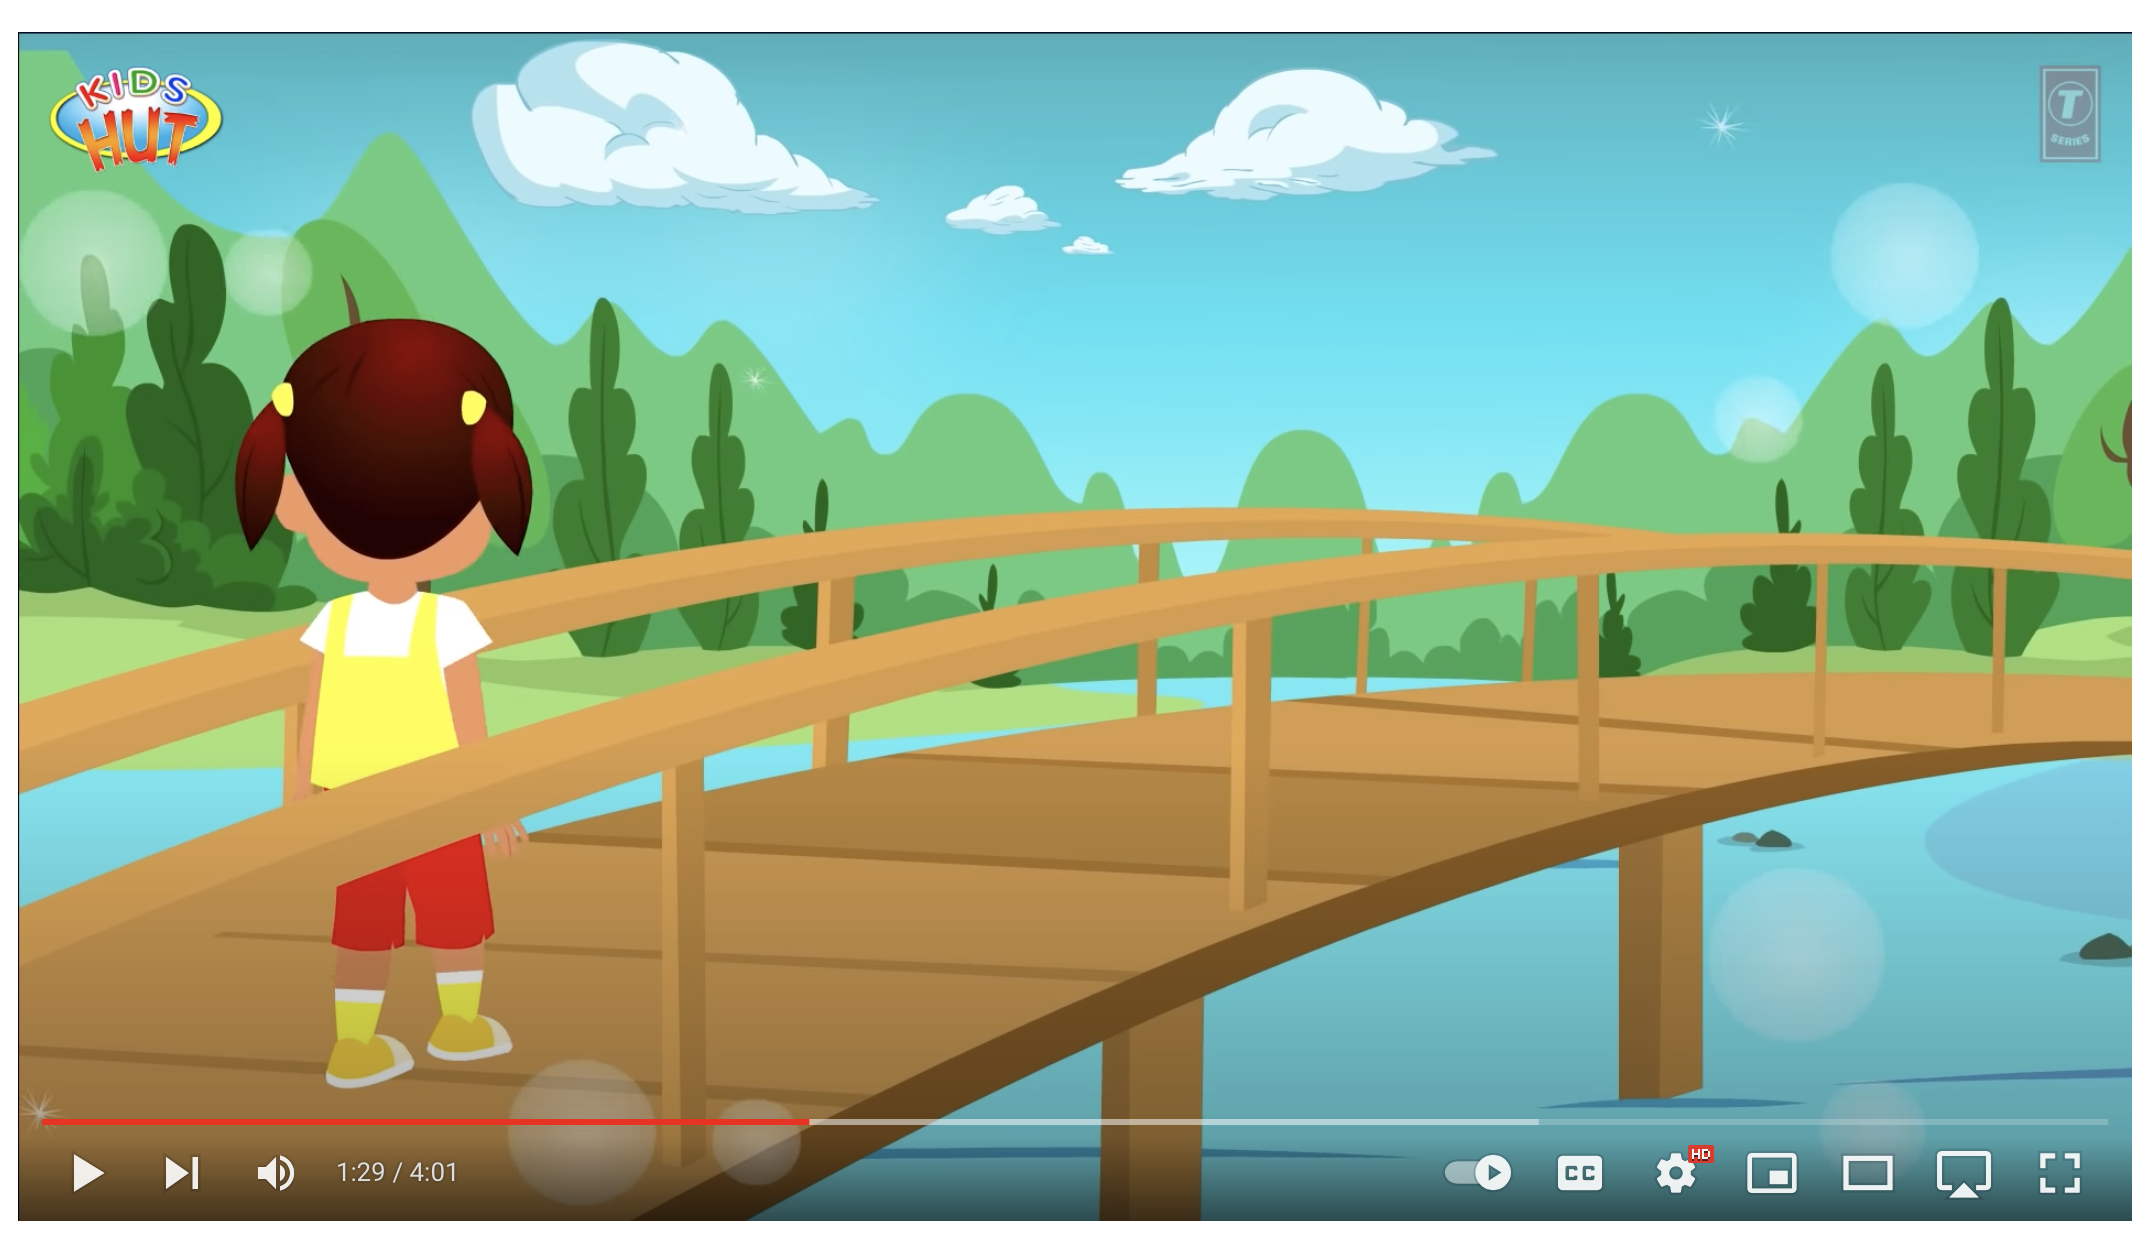}
    \caption[Visual labeling]{An example of a video frame with information present in visual modality to answer questions. The question asked in this frame is: `What is used to cross a river?' }
    \label{fig:visual_example}
\end{figure}

\begin{figure}[htb!]
    %\centering
    \includegraphics[scale=0.2]{./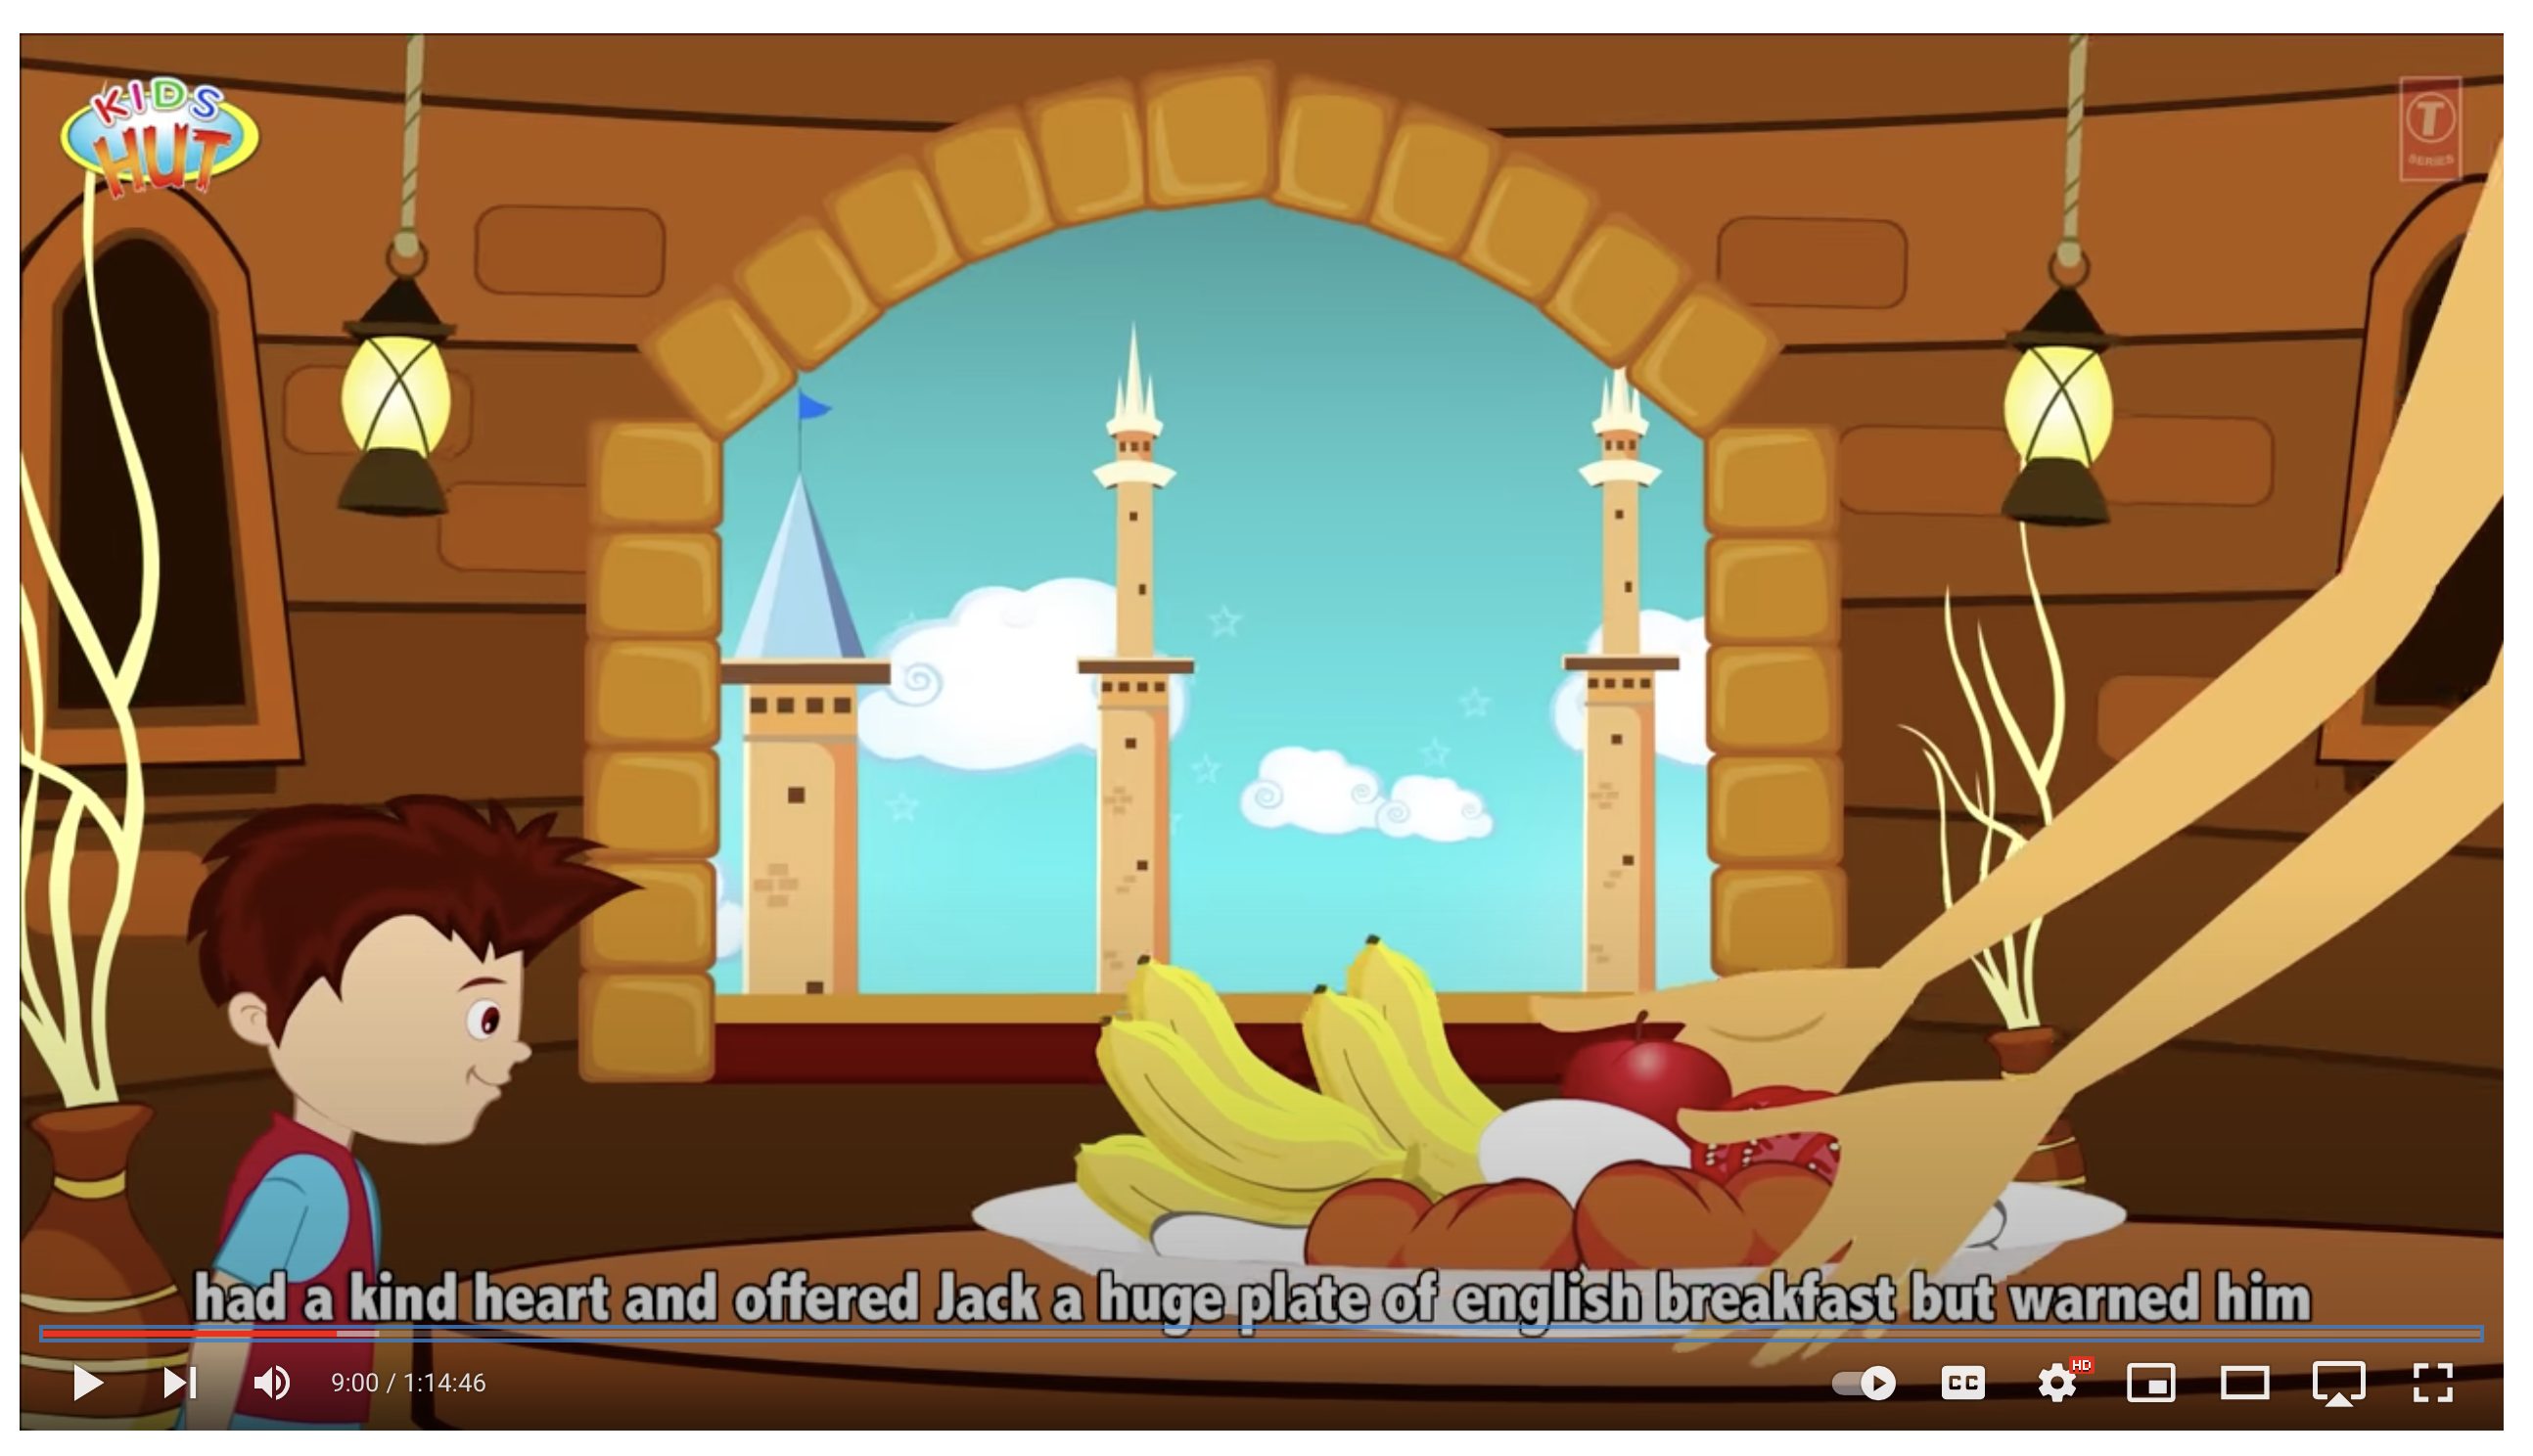}
    \caption[Visual labeling]{An example of a video frame with information in both language and visual modality to answer questions. The question asked in this frame is: `What is included in an English breakfast?' }
    \label{fig:dual_example}
\end{figure}

As mentioned earlier, only one labeler labeled each video as video labeling is a very time and effort-intensive exercise. Moreover, the aim is not to get the highest recall for questions but to find if factual question-answers are present in the video and if an RC model could answer such questions.

\section{Additional Details on Error Cases}
We provide additional examples of the error cases to better understand when the RC model is making mistakes. We also provide additional examples of cases when the models work. In Fig.~\ref{fig:error_cases2} and Fig.~\ref{fig:error_cases3}, we show two examples of mistakes by the RC models. We find that in case videos have animations (or cartoons), the visual information is not captured in the captions, leading to more mistakes. In Fig.~\ref{fig:good_cases}, we present examples that show that the RC models work well when the answer is directly present in the context text. However, the model makes mistakes more often for complex questions requiring multiple sentences to be analyzed.

\begin{figure}[htb!]
    %\centering
    \includegraphics[scale=0.30]{./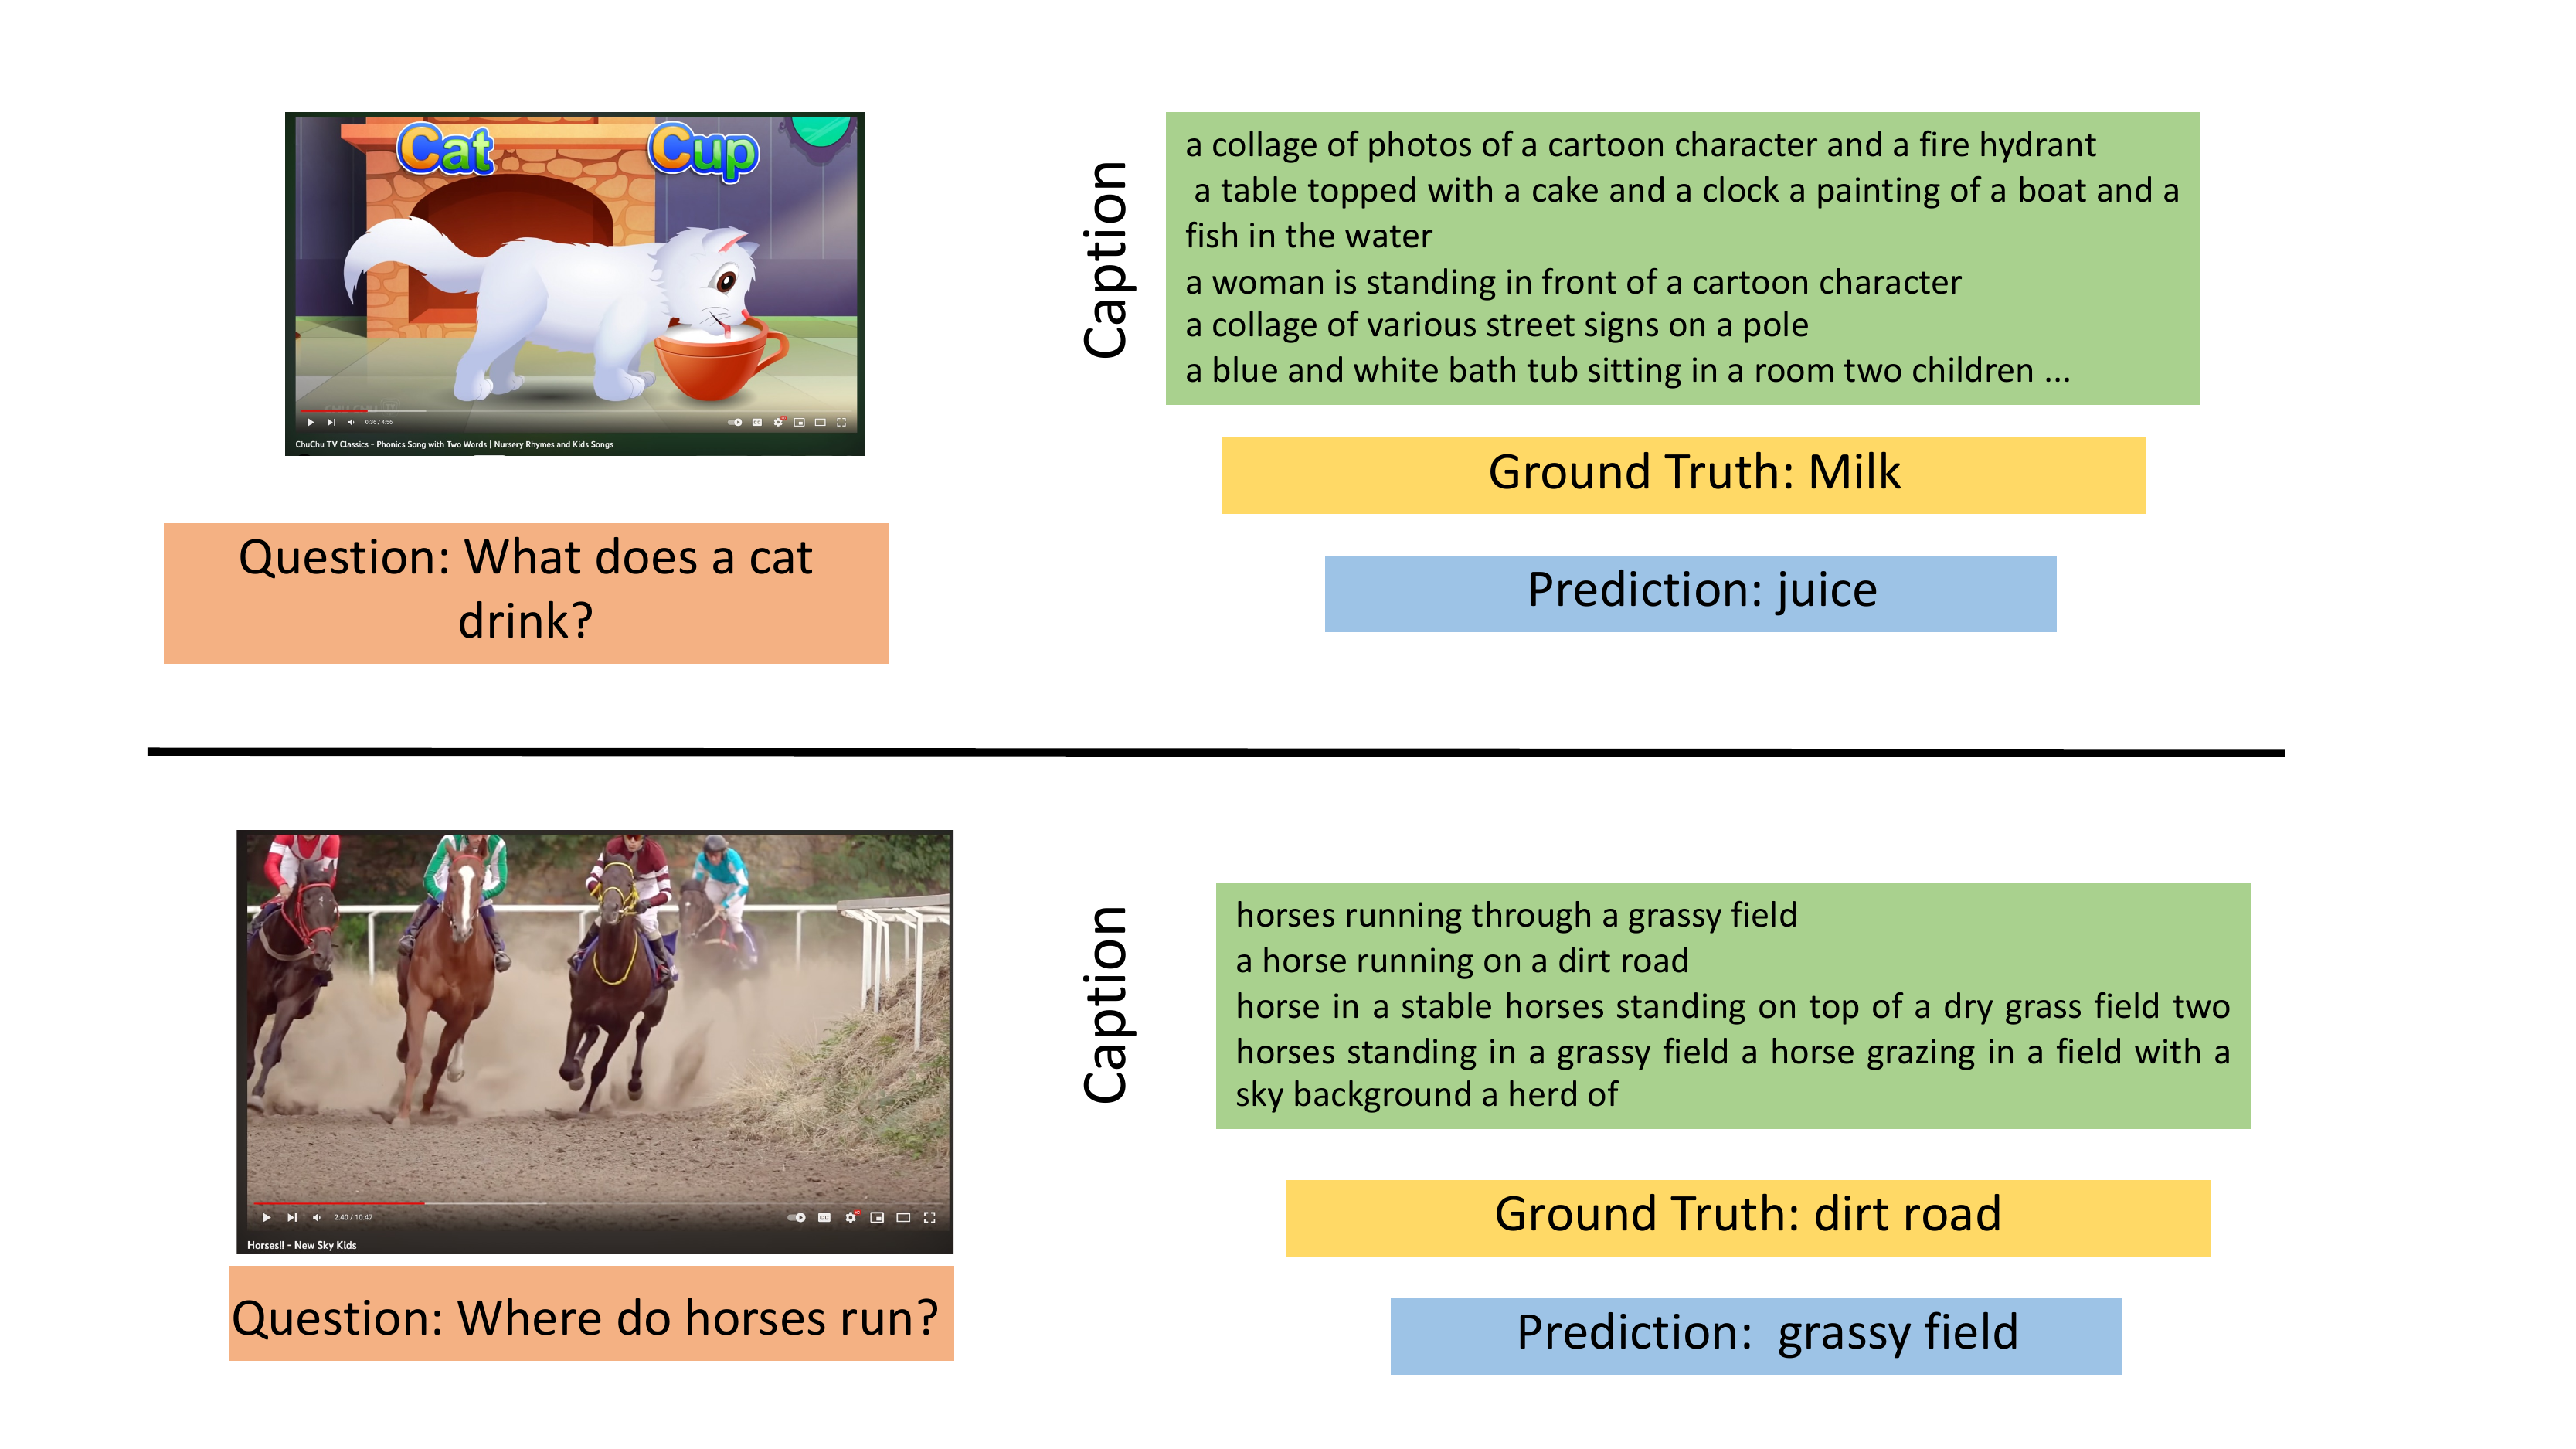}
    \caption[RC Model]{Examples of incorrect predictions by the Longformer model when using video frame captions. }
    \label{fig:error_cases2}
\end{figure}

In Fig.~\ref{fig:error_cases2}, we show two examples of visual information used to derive questions. In the top figure, it is apparent that the cat is drinking milk. However, the RC prediction was incorrect as the caption could not include information about the cat and the mils, leading to a random prediction. While in real-life images with cats, a good captioning model can extract the information about the cat, in the case of cartoon images, detecting a cat could be a challenge. In the bottom example, the captioning system generates two similar examples of captions  horses running through a grassy filed', and  `a horse running on a dirt road'. When asked where horses run, the RC model likely uses the first caption information that is incorrect.

\begin{figure}[htb!]
    %\centering
    \includegraphics[scale=0.30]{./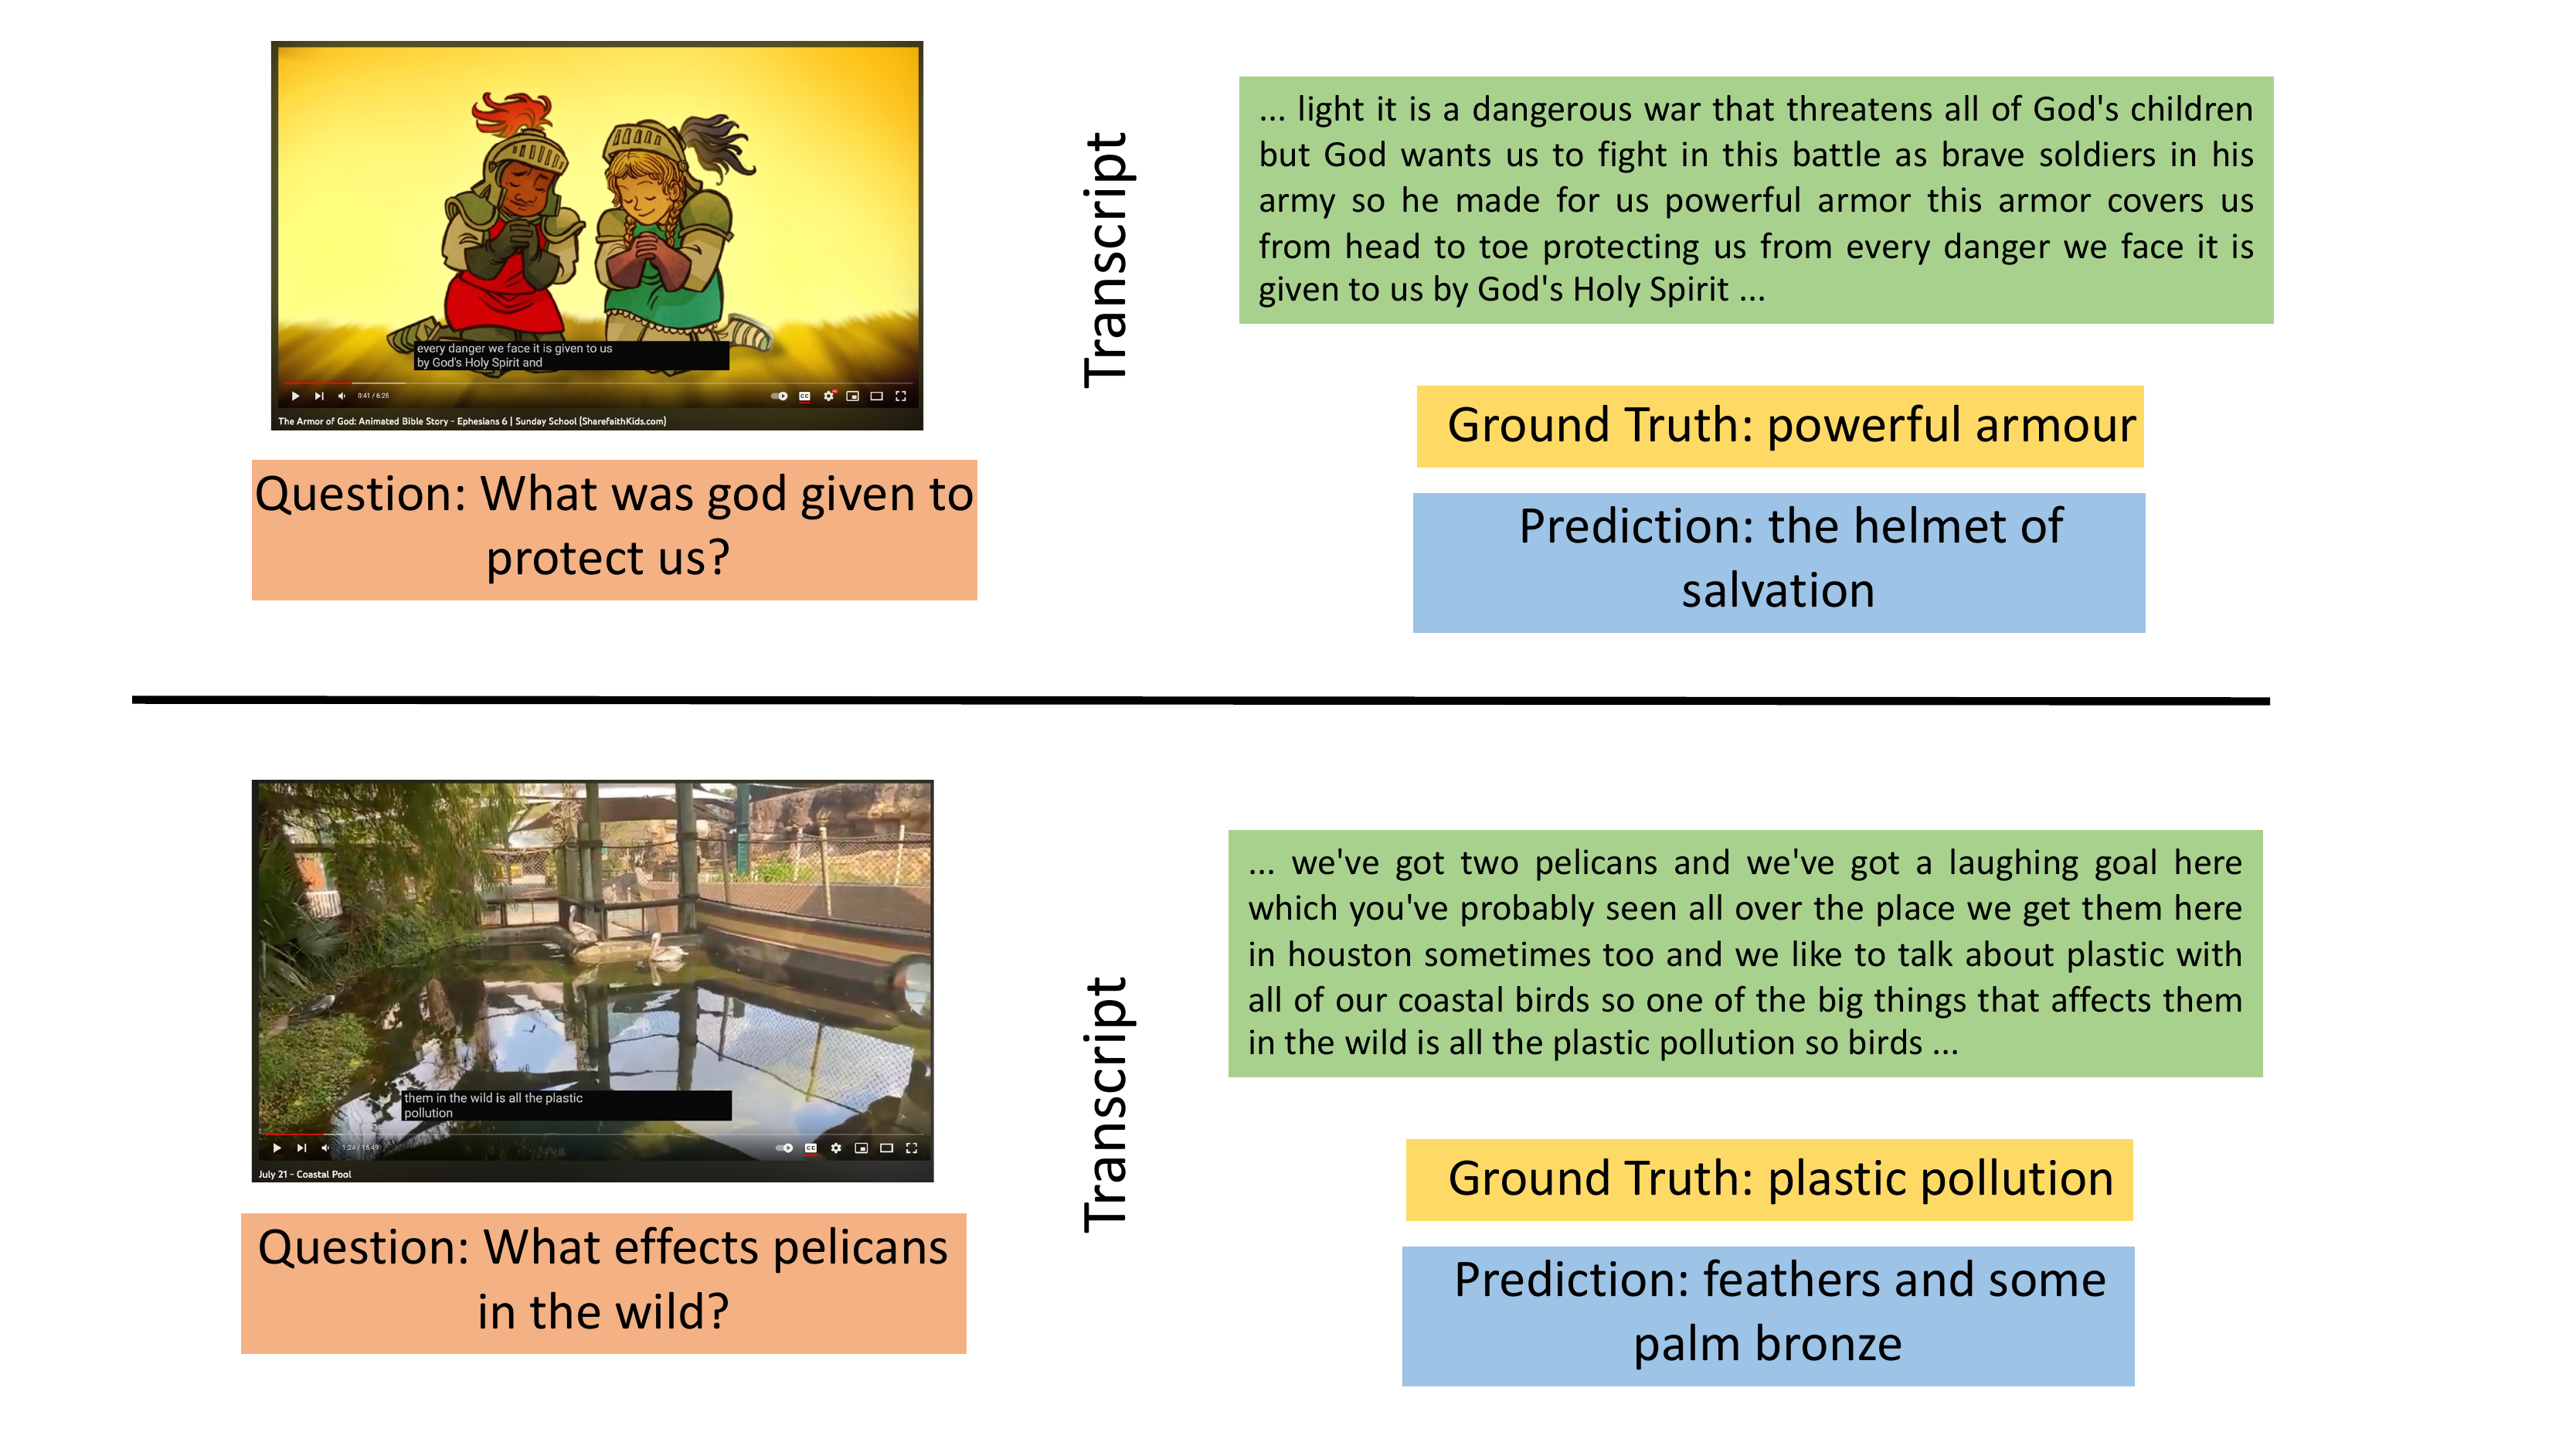}
    \caption[RC Model]{Examples of incorrect predictions by the Longformer model when using video transcripts. }
    \label{fig:error_cases3}
\end{figure}

In Fig.~\ref{fig:error_cases3}, we show two examples of audio information (showing video transcript) getting used to derive questions. In the top figure, the statements are rather abstract and confounded. When a question is posed on `What has god given to protect us?', the model generates a random output not present in the video. A similar issue could be noted for the bottom figure.

\begin{figure}[htb!]
    %\centering
    \includegraphics[scale=0.30]{./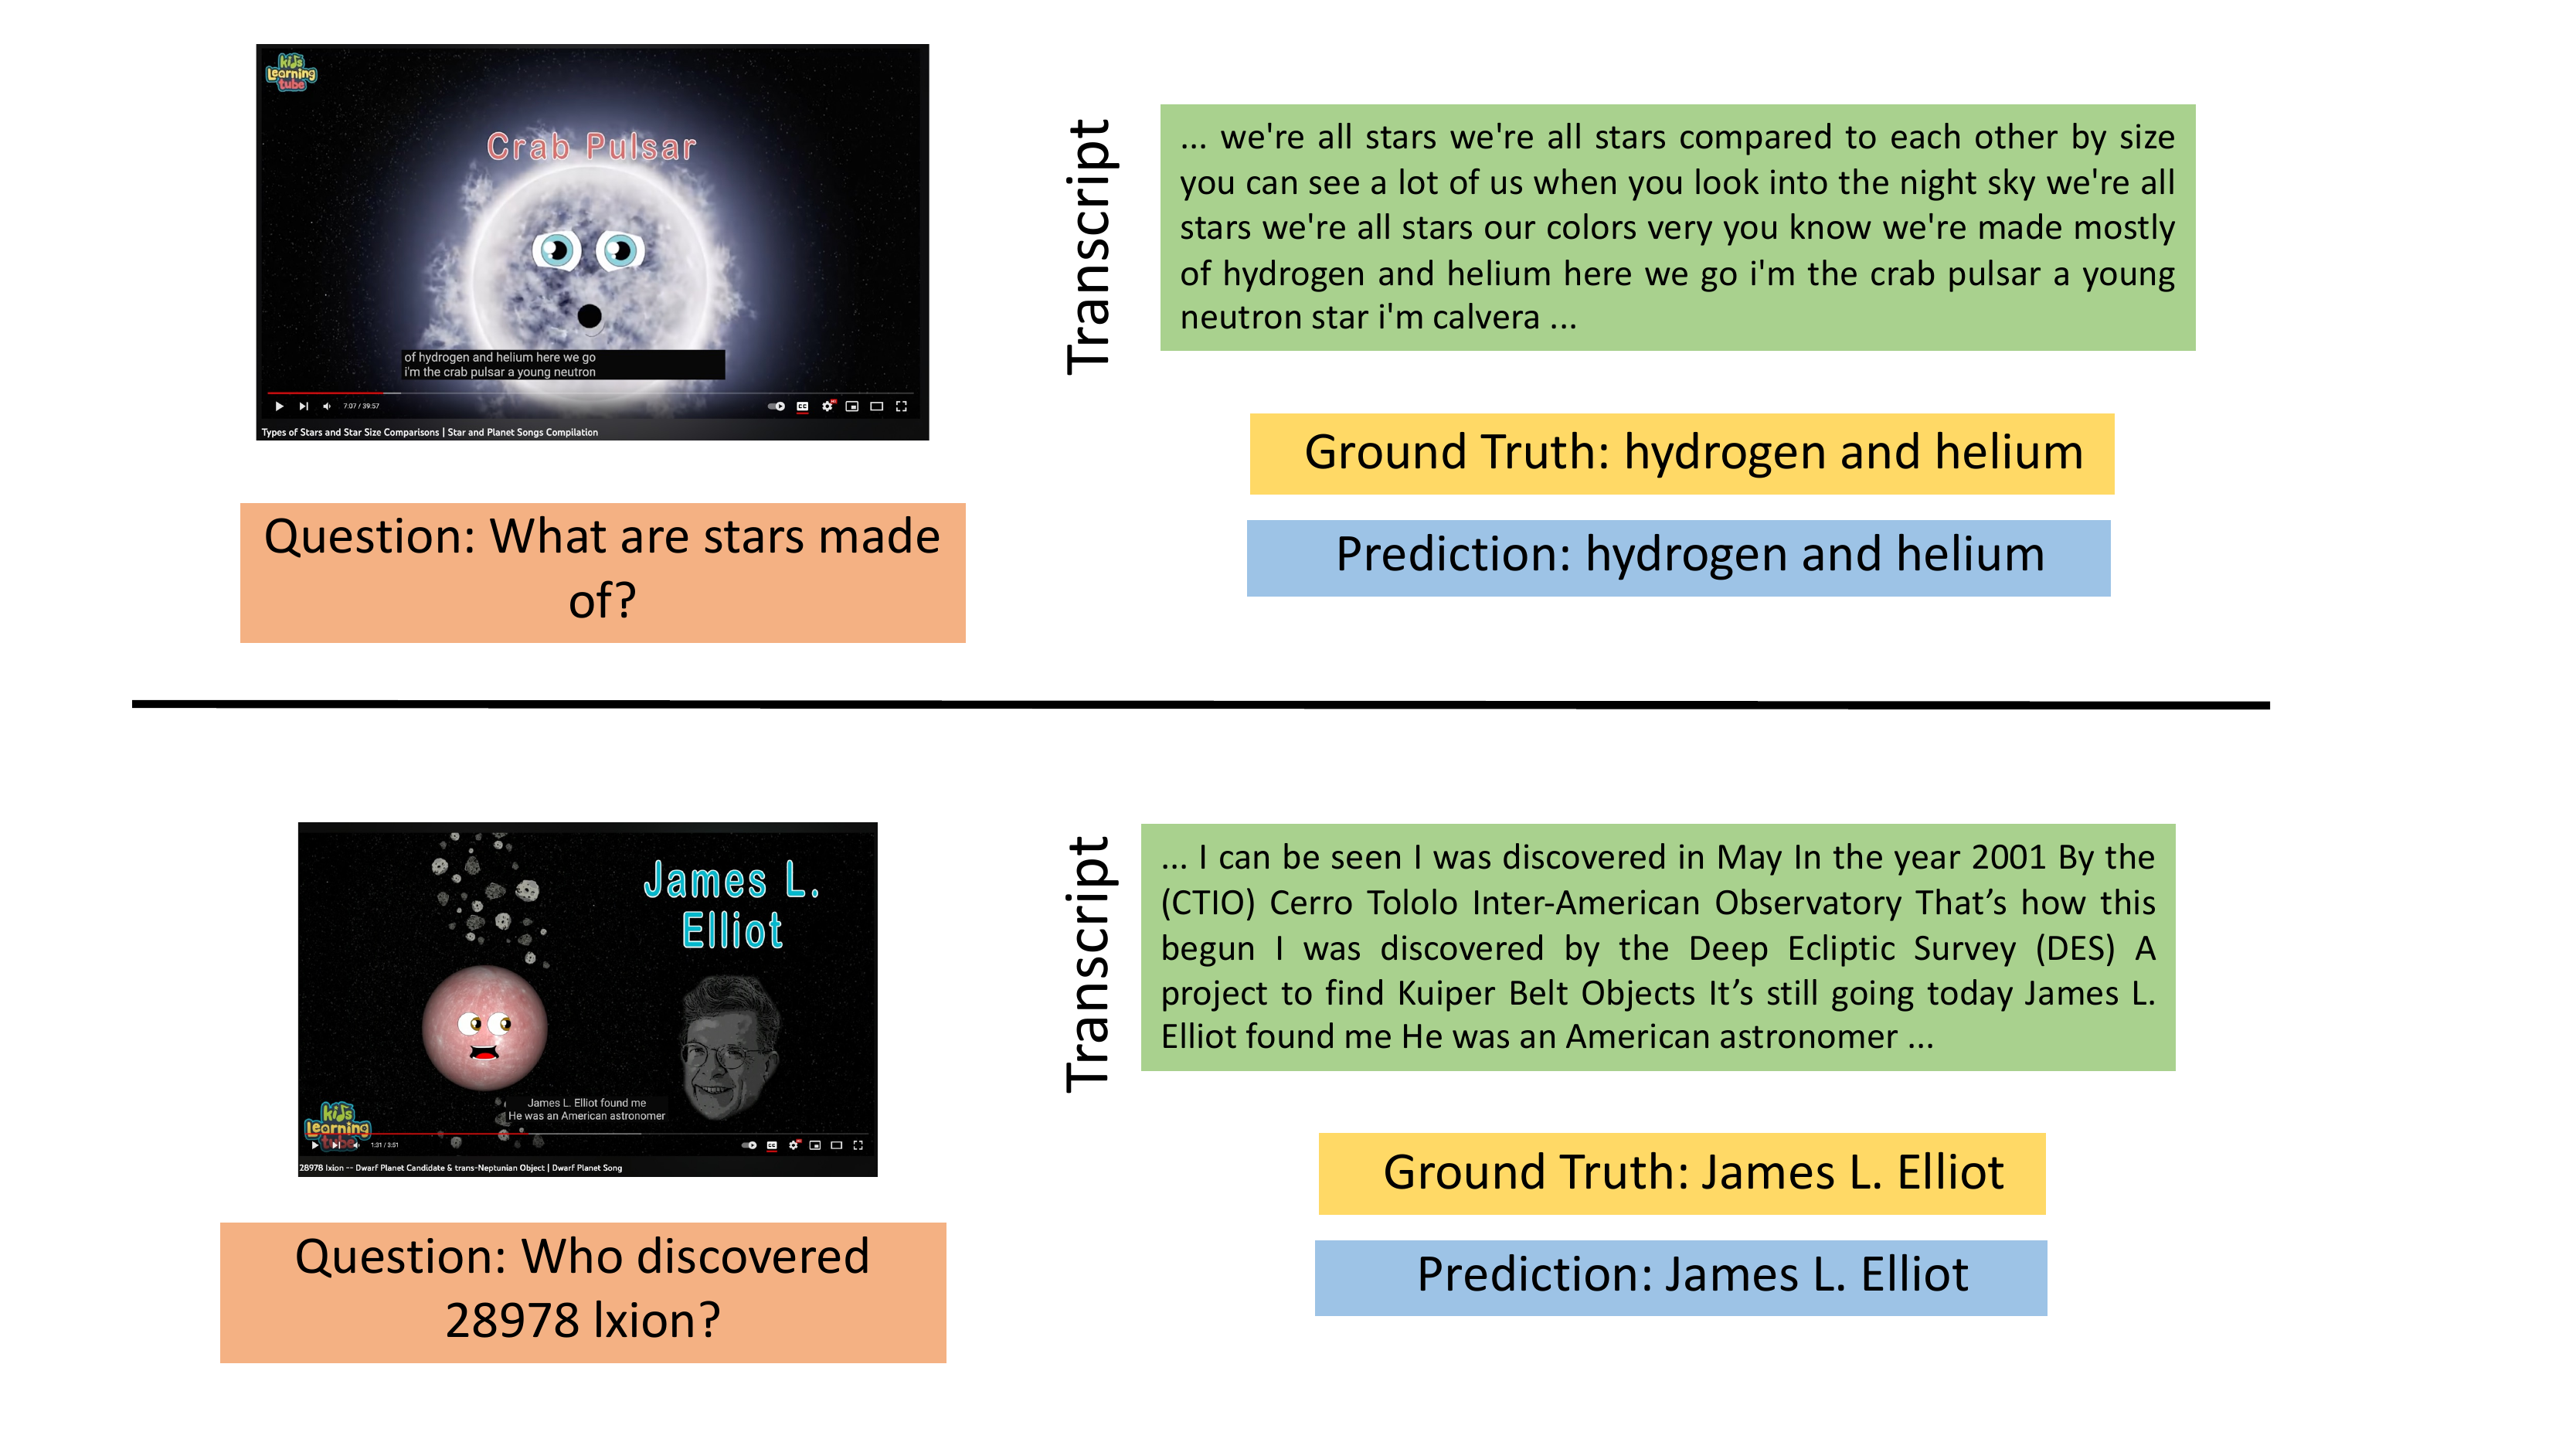}
    \caption[RC Model]{Examples of correct predictions by the Longformer model when using video transcripts. }
    \label{fig:good_cases}
\end{figure}

In Fig.~\ref{fig:good_cases}, there are two additional cases when the model has made correct predictions. In both cases, the expected answers were present in the video transcript, and the questions were not complex. Also, the questions are factual and have straightforward answers.

Using these few instances of manual verification, we find that captions quality is not good in all cases, especially when the video frames have animations or cartoons. Poor captioning leads to many mistakes. We also find that the model performs well for factual questions with straightforward answers in the video transcript. The model performs poorly when questions are more involved and require combining words from multiple sentences.

\section{Additional Details on Videos Dataset}
Here we provide details on all YouTube channels used for this research. As mentioned earlier, the channels were obtained based on the rank provided by the Social Blade website, which maintains the ratings of many YouTube channels for different categories. Table~\ref{tab:channels1} and Tab.~\ref{tab:channels2} provide information on  `Channel Name' , `Channel Views'  and `Channel Subscribers'. The `Number of Videos' tells the videos we can use for this analysis. The table rows are sorted in reverse order of the number of videos present for each channel. 

We only limited our analysis to the top channels (because of computational constraints). Moreover, not all channels have video transcripts (retrieval via YouTube API). We only used videos with video transcripts, and we could download the videos to extract the frames. Moreover,  However, the top channels receive a substantial fraction of the total views, so our analysis is based on videos that reach millions of children.  The approach is generalizable as it only requires video data and therefore could easily be extended to additional channels. 

\begin{table}[ht!]
\scriptsize
\caption{YouTube Kids Videos Dataset - Part 1: A sample list of YouTube channels considered in this study. Overall top 100 channels were used for the analysis. Channel statistics reflect data as on  20 Jan 2022.}
\centering

 \begin{tabular}{|p{2.5cm}|p{1.0cm}|p{1.0cm}|p{0.5cm}|} 
 \hline
 Channel Name & Channel Views & Channel Subscribers  & \# of Videos  \\ [0.5ex] 
 \hline
 \hline
 
 Jugnu Kids - Nursery   Rhymes and Best Baby Songs & 4B & 10M & 4676 \\ \hline
Toys And Funny Kids Play Doh Cartoons & 3B & 9M & 4381 \\ \hline
PowerKids TV & 17B & 33M & 4223 \\ \hline
King Games & 2B & 3M & 4044 \\ \hline
WildBrain Kids & 2B & 6M & 3990 \\ \hline
Kids TV - Nursery Rhymes And Baby Songs & 12B & 21M & 3635 \\ \hline
Sesame Street & 21B & 23M & 3564 \\ \hline
HobbyFamilyTV & 8B & 4M & 3493 \\ \hline
Cartooning Club How to Draw & 992M & 4M & 3367 \\ \hline
Tayo the Little Bus & 7B & 9M & 3099 \\ \hline
CBC Kids & 70M & 105K & 3090 \\ \hline
Pinkfong Baby Shark - Kids' Songs \&   Stories & 36B & 65M & 2648 \\ \hline
KidsBabyBus HD & 1B & 2M & 2400 \\ \hline
Kids Channel - Cartoon Videos for Kids & 3B & 6M & 2380 \\ \hline
Ryan's World & 54B & 34M & 2322 \\ \hline
AllToyCollector & 1B & 1M & 2210 \\ \hline
Shemaroo Kids & 3B & 8M & 2144 \\ \hline
BabyBus - Kids Songs and Cartoons & 25B & 31M & 2001 \\ \hline
SimpleCrafts - 5 Minute Crafts For All & 214M & 729K & 1441 \\ \hline
Little Treehouse Nursery Rhymes and Kids   Songs & 5B & 10M & 1430 \\ \hline
Polly Pocket & 813M & 1M & 1273 \\ \hline
Kids Toys Play & 636M & 541K & 1164 \\ \hline
Geethanjali Kids - Rhymes and Stories & 583M & 1M & 1106 \\ \hline
Onyx Family & 2B & 3M & 1098 \\ \hline
T-Series Kids Hut & 969M & 2M & 1053 \\ \hline
Yo Gabba Gabba! - WildBrain & 1B & 1M & 1000 \\ \hline
Fun Kids Planet & 828M & 1M & 998 \\ \hline
Team BBB & 3M & 10K & 982 \\ \hline
Houston Zoo & 19M & 49K & 915 \\ \hline
Cupcake Squad & 879M & 1M & 866 \\ \hline
Cocomelon - Nursery Rhymes & 152B & 155M & 862 \\ \hline
HooplaKidz TV - Funny Cartoons For Kids & 1B & 3M & 848 \\ \hline
Dream English Kids & 2B & 3M & 767 \\ \hline
WonderBalls - Official Channel & 210M & 395K & 758 \\ \hline
Arts and Crafts For Toddlers! & 44M & 5M & 691 \\ \hline
Super Simple Songs - Kids Songs & 41B & 37M & 667 \\ \hline
Videogyan Kids Shows-Children's Cartoon   Animation & 4B & 8M & 667 \\ \hline
Busy Beavers - Kids Learn ABCs 123s \&   More & 3B & 3M & 662 \\ \hline
BillionSurpriseToys - English Kids Songs   \& Cartoon & 8B & 50M & 649 \\ \hline
FitDance Kids \& Teen & 670M & 1M & 648 \\ \hline
Cosmic Kids Yoga & 357M & 1M & 646 \\ \hline
Kids Learning Videos & 969M & 669K & 633 \\ \hline
LooLoo Kids - Nursery Rhymes and   Children's Songs & 31B & 52M & 621 \\ \hline
Liberty's Kids - WildBrain & 36M & 169K & 608 \\ \hline
MagicBox English & 526M & 919K & 604 \\ \hline
Super Crazy Kids & 4B & 9M & 595 \\ \hline
N3ON & 32M & 479K & 577 \\ \hline
 \end{tabular}
\label{tab:channels1}
\end{table}

\begin{table}[ht!]
\scriptsize
\caption{YouTube Kids Videos Dataset - Part 2: A sample list of YouTube channels considered in this study. Overall top 100 channels were used for the analysis. Channel statistics reflect data as on  20 Jan 2022.}
\centering

 \begin{tabular}{|p{2.5cm}|p{1.0cm}|p{1.0cm}|p{0.5cm}|} 
 \hline
 Channel Name & Channel Views & Channel Subscribers  & \# of Videos  \\ [0.5ex] 
 \hline
 \hline

TOP BEST APPS FOR KIDS & 532M & 662K & 564 \\ \hline
ChuChu TV Nursery Rhymes \& Kids Songs & 42B & 62M & 547 \\ \hline
The Influencer Family & 1M & 12K & 532 \\ \hline
New Sky Kids & 1B & 2M & 511 \\ \hline
KLT & 1B & 1M & 508 \\ \hline
Kids TV Play Doh - How to DIY & 95M & 157K & 506 \\ \hline
Moose Top TV Commercials & 890M & 67K & 493 \\ \hline
3KidsTV & 1M & 9K & 483 \\ \hline
Top Best Apps Planet & 44M & 87K & 478 \\ \hline
Kids Activities & 3M & 13K & 455 \\ \hline
My Kids Rhymes & 14M & 50K & 445 \\ \hline
KID-A-LOO & 5M & 17K & 409 \\ \hline
Kyoot & 1B & 5M & 383 \\ \hline
Hillsong Kids & 36M & 187K & 378 \\ \hline
Baby Einstein & 670M & 838K & 352 \\ \hline
GiggleBellies - Colorful Toddler Learning   Videos & 914M & 671K & 343 \\ \hline
3ABN Kids Network & 3M & 21K & 323 \\ \hline
Dinosaur Patrol & 22M & 32K & 316 \\ \hline
Kids Channel - Learn with Fun & 1M & 10K & 293 \\ \hline
Mini Pop Kids & 59M & 243K & 280 \\ \hline
Sharefaith Kids & 18M & 131K & 274 \\ \hline
Tic Tac Toy & 3B & 5M & 265 \\ \hline
Smighties & 30M & 65K & 262 \\ \hline
ChuChuTV Police \& Surprise Eggs & 4B & 7M & 254 \\ \hline
ChuChuTV Storytime for Kids & 1B & 2M & 253 \\ \hline
Jaz Toonz TV - Cartoon Kids Shows \&   Nursery Rhymes & 106M & 324K & 249 \\ \hline
Moose Toys & 192M & 116K & 248 \\ \hline
Elizabeth \& Eva TV & 42M & 169K & 239 \\ \hline
Little Tritans - Kids Songs and Nursery   Rhymes & 871M & 1M & 223 \\ \hline
DJC Kids & 212M & 245K & 215 \\ \hline
Kids World & 75K & 1K & 209 \\ \hline
Debbie Doo Kids TV & 1B & 1M & 170 \\ \hline
Little Smart Kids & 228M & 261K & 156 \\ \hline
ESL Kids Games & 6M & 70K & 143 \\ \hline
Lalay Kids Tv - Colors, Stories Read   Aloud & 1M & 3K & 136 \\ \hline
ZJfun & 38K & 936 & 131 \\ \hline
Rapid Kids TV & 204M & 849K & 129 \\ \hline
Two Kids TV & 153M & 304K & 115 \\ \hline
Foal On The Roll & 782K & 1K & 115 \\ \hline
Bellboxes & 147M & 205K & 101 \\ \hline
Super Cars Cartoon & 432M & 1M & 99 \\ \hline
Marcelo Toys \& More & 590K & 4K & 96 \\ \hline
Can Cubs Educational Centre & 667K & 746 & 93 \\ \hline
AM Kids & 2M & 17K & 92 \\ \hline
H\&Z Family Show & 258K & 7K & 88 \\ \hline
VenturesFamily & 724K & 2K & 85 \\ \hline
Vivan Malhotra & 253K & 800 & 67 \\ \hline
KIDS ZONE TV RHYMES & 352K & 1M & 67 \\ \hline
Funny Kids Playtime with Jade \& James   - ToysReview & 154K & 1K & 65 \\ \hline
Jelly Kids Tv HD & 41K & 372 & 65 \\ \hline
English Paradise Kids & 199M & 122K & 62 \\ \hline
Hunter and Adventures & 58K & 370 & 57 \\ \hline
 \end{tabular}
\label{tab:channels2}
\end{table}
